# Supplementary material for: From Planar Solitons to Vortex Rings and Lines: Cascade of Solitonic Excitations in a Superfluid Fermi Gas
Source: arXiv:1507.01047 source file (2015-07-03)

a

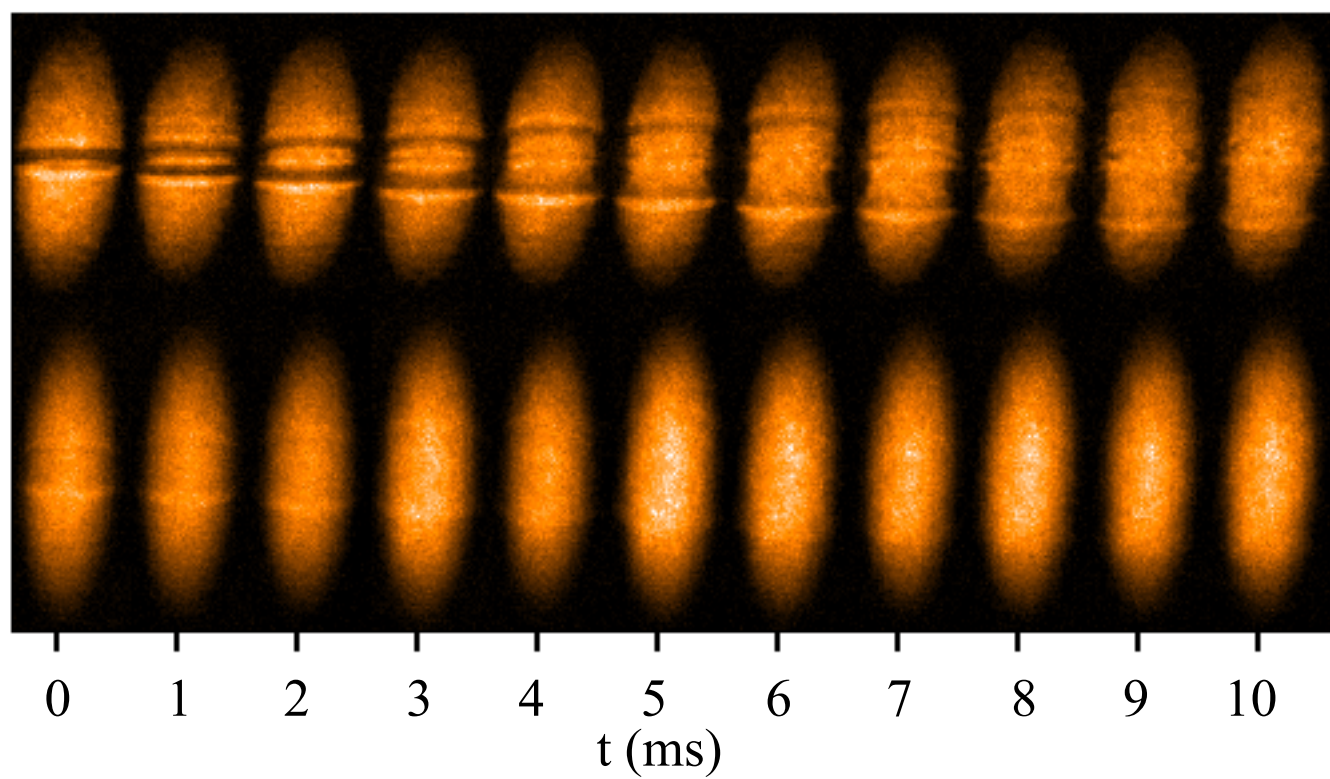

b

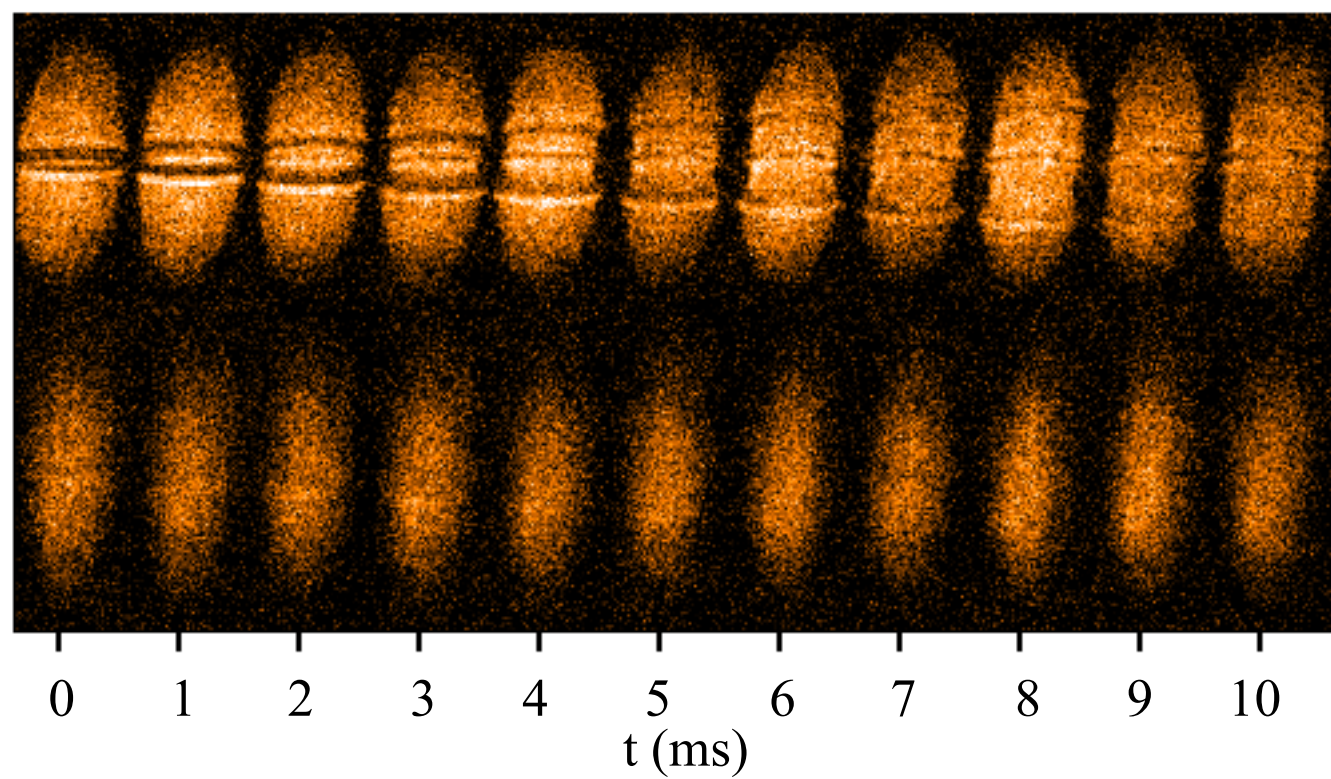

a

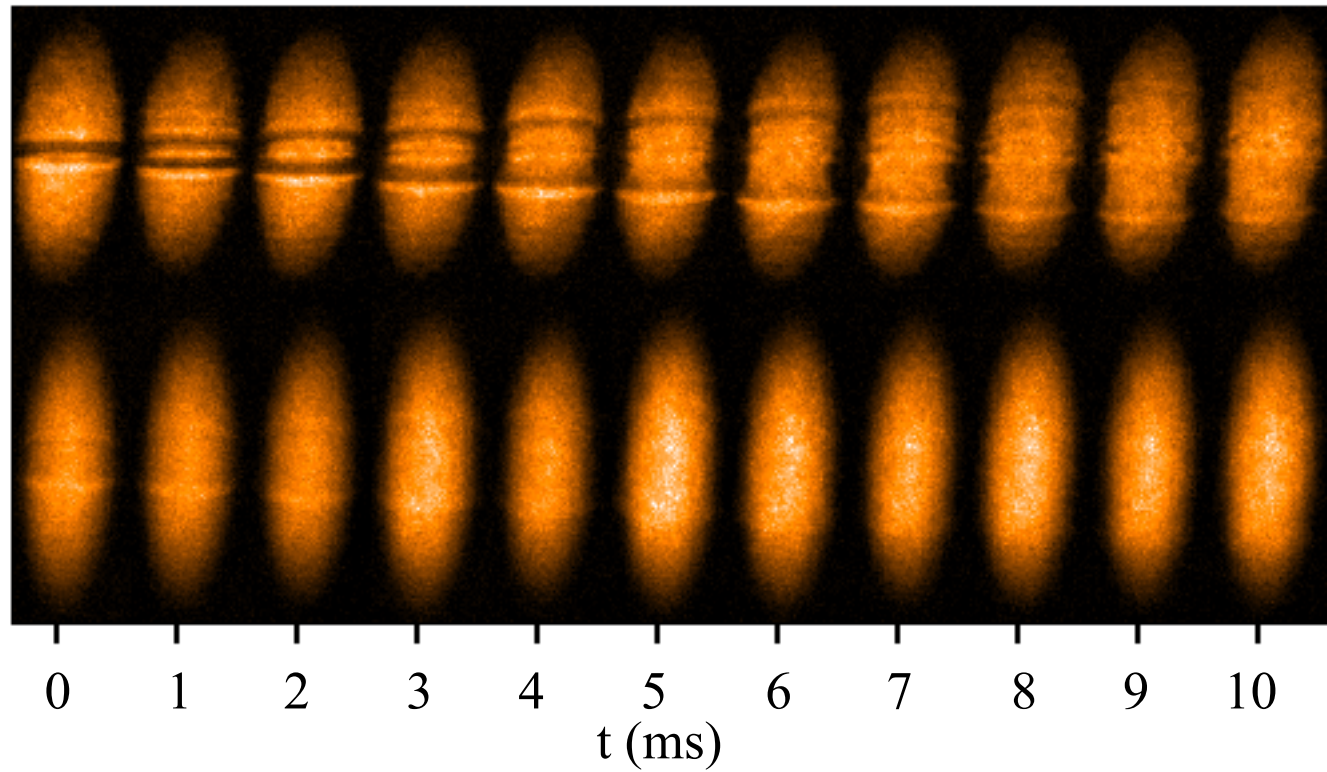

b

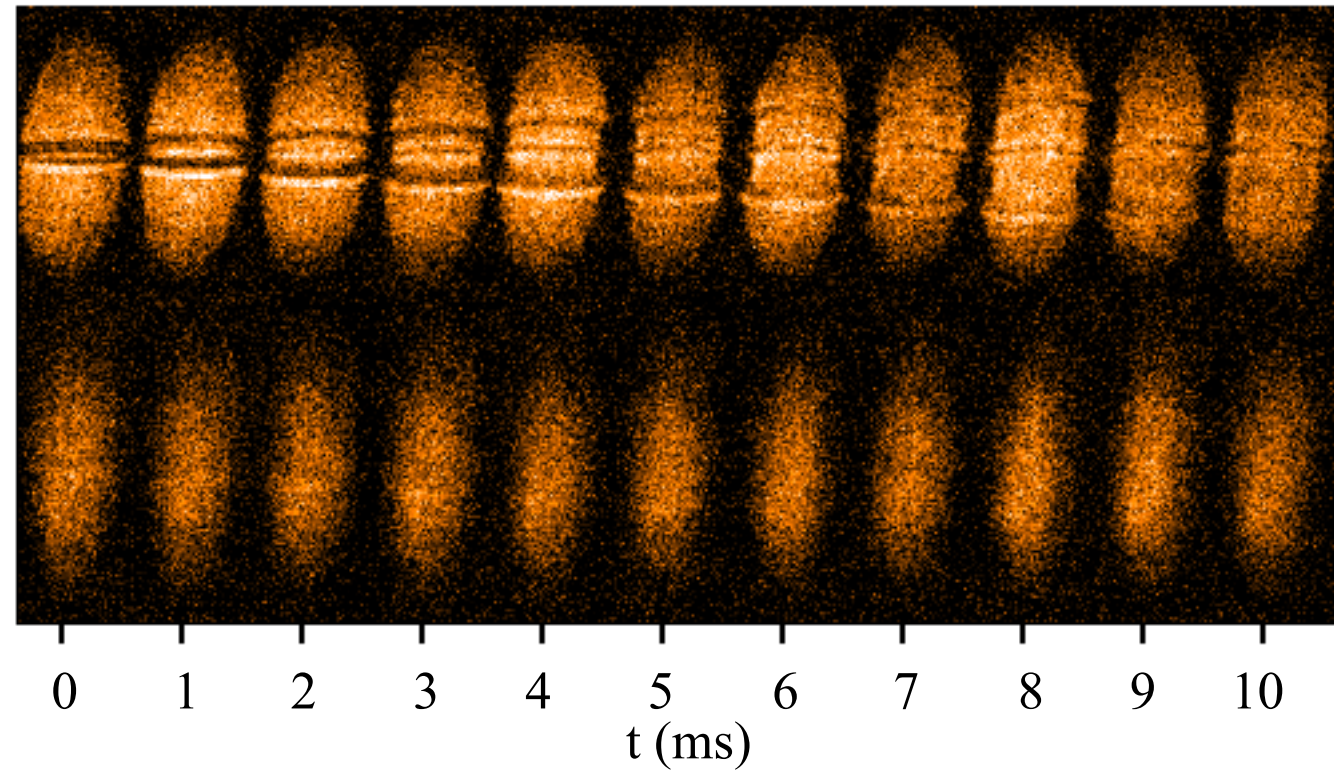

Supplement: Supplementary file 1 [file SuppFig_RapidRampComparison.pdf]
